# Supplementary material for: Kairos: Practical Intrusion Detection and Investigation using Whole-system Provenance
Source: arXiv:2308.05034 source file (2023-09-28)
Supplement: Supplementary file 1 [file appendix_optc.tex]

We evaluated \system
on a subset of DARPA's OpTC data %
to provide some preliminary experimental results.
The OpTC dataset is large,
containing benign activities of $500$ Windows hosts
over the course of seven days
(September 17 - 23, 2019)
and additional three days 
(September 23 - 25, 2019)
of a mixture of benign and APT activities.
The red team simulated a three-day long
APT attack
using a number of known CVEs
(\ie CVE-2021-30551,
CVE-2020-0688, and 
CVE-2019-0604)
on a small subset
of hosts (approximately $10$).
Due to time constraints\footnote{The total size of the dataset is in the order of a few dozen TBs.} of the rebuttal,
we selected only one host (\texttt{Sysclinet0201})
that was involved in the attack
to report our preliminary experimental results.
We used the benign data
from September 19 to September 21 
for training,
September 22's benign data
for validation (\ie to set thresholds),
and September 23's data
(which contains both benign and attack activity)
for testing.
Note that the data from
September 23
contains \emph{all} the malicious activity
of \texttt{Sysclinet0201},
because that host was no longer involved
in the APT in the remaining two attack days.
However,
only a subset of the host's benign data
is used for training;
whether this subset of data is representative
of the host's normal behavior is unknown to us,
since the dataset is poorly documented.
We analyzed a total of $358.7$ GB of data
and labeled the data in the same way
as in the DARPA TC experiments (\autoref{sec:evaluation:datasets:darpa}).
We used the same default hyperparameters
($|\Phi|$ = $16$,
$|\mathbf{s}(v)| = 100$,
$|\mathcal{N}| = 20$,
$|\mathbf{z}| = 200$,
$|\mathbf{tw}| = 15$ minutes)
as described in~\autoref{sec:evaluation}.
\autoref{tab:evaluation:optc_datasets}
reports the same graph statistics
as in~\autoref{tab:evaluation:datasets}.
Note that
due to lack of documentation,
the number of total attack edges
is only a rough, conservative estimate;
the actual number might be larger.

\begin{table}[t]
\caption{Summary of OpTC dataset. }
\label{tab:evaluation:optc_datasets}
\resizebox{\columnwidth}{!}{%
  \begin{tabular}{|l|l|l|l|l|}
    \hline
    \textbf{Dataset} &
    \textbf{\# of Nodes} &
    \textbf{\begin{tabular}[c]{@{}c@{}}\# of Edges \\ (in millions)\end{tabular}} &
    \textbf{\begin{tabular}[c]{@{}c@{}}\# of Attack \\ Edges\end{tabular}} &
  \textbf{\begin{tabular}[c]{@{}c@{}}\% of Attack \\ Edges\end{tabular}} \\ %
    \hline
    DARPA-OpTC & 692,531 & 19.0 & 2,684 & 0.014\% \\ %
    \hline
  \end{tabular}
}
\end{table}

\begin{figure}[h]
	\centering
	\includegraphics[width=\columnwidth]{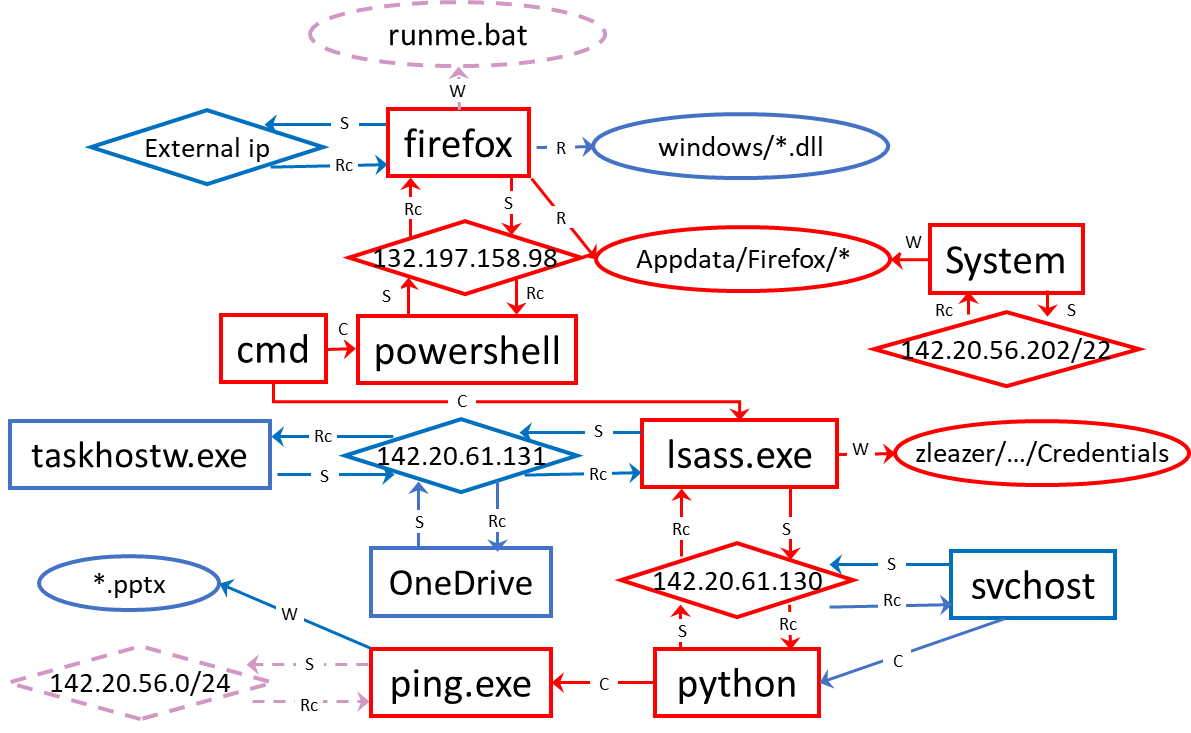}
	\caption{A \change{summary} graph that describes attack activity in DARPA's OpTC dataset, as automatically generated by \system. 
	Colors and dashed elements are added to ease comparison with the ground truth.}
	\label{fig:evaluation:casestudy_optc}
\end{figure}

\system achieves $88.3\%$ accuracy,
reporting no false-negative time windows
and only $7$ false-positive windows;
therefore,
the preliminary results are comparable 
to DARPA TC's 
experimental results (\autoref{tab:evl:exp}).
\autoref{fig:evaluation:casestudy_optc} is 
a candidate summary graph
that describes
the APT activity in the OpTC experiment.
We manually translate the ground truth logs
to attack edges,
but our observation of \system' reconstructed
attack graph leads us to believe that
the ground truth documentation may be incomplete.
For example,
\texttt{svchost} (a shell for loading DLL files)
communicated with
an attacker's IP (\texttt{142.20.61.130}),
but this activity was not mentioned
in the ground truth.

\begin{figure}[h]
	\centering
	\includegraphics[width=\columnwidth]{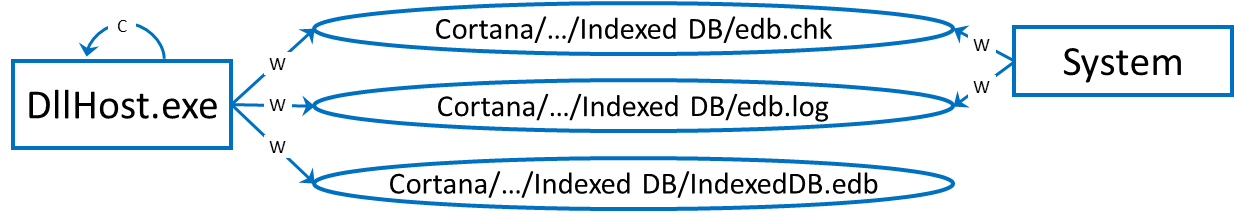}
	\caption{A benign \change{summary graph} in DARPA's OpTC dataset.}
	\label{fig:evaluation:casestudy_benign_optc}
\end{figure}

\autoref{fig:evaluation:casestudy_benign_optc}
is a benign summary graph
describing a system update on Cortana,
Windows' virtual assistant program.
\system considered it to be suspicious,
because such an activity did not appear in the training data.
We discuss in~\autoref{sec:evaluation:detection}
how \system can readily address this problem.

We will conduct a more thorough evaluation
of \system on the OpTC dataset
in the revised paper.
